# Supplementary material for: Test of lepton flavor universality with $\bar{B} \rightarrow D^{(*)} \tau^{-} \bar{\nu}_{\tau}$ and $\bar{B} \rightarrow D^{(*)} \ell^{-} \bar{\nu}_{\ell}$ decays at Belle II
Source: arXiv:2609.21947 source file (2026-09-18)
Supplement: Supplementary file 1 [file suppldefinitions.tex]

\usepackage[dvipdfmx]{graphicx} % Include figure files

% Packages
\usepackage{wrapfig}
\usepackage[caption=false]{subfig}
\usepackage{epstopdf} % Allow to include eps files
\usepackage{xcolor} % Color support
\usepackage{amssymb} % Extended symbol collection
\usepackage{hyperref} % Generate pdfs with hyperlinks
\usepackage[utf8]{inputenc} % Allow UTF8 characters
\usepackage[english]{babel} % All publications are in English
\usepackage{blindtext} % For testing
\usepackage{subfiles}
\usepackage{multirow}
\usepackage{booktabs}
\usepackage{bm}
\usepackage{cases}
\usepackage {autobreak}
\usepackage{tabularx}
\usepackage{comment}
\usepackage{orcidlink} % for ORCIDs in author list

% Configuration
\graphicspath{{SupplFigures/}} % Use Figures directory for figures

% Usual (decimal) numbering
\renewcommand{\thesection}{\arabic{section}}
\renewcommand{\thesubsection}{\thesection.\arabic{subsection}}
\renewcommand{\thesubsubsection}{\thesubsection.\arabic{subsubsection}}

% Fix references
\makeatletter
\renewcommand{\p@subsection}{}
\renewcommand{\p@subsubsection}{}
\makeatother

% Numbering
%\renewcommand{\theequation}{\arabic{section}.\arabic{equation}}
%\renewcommand{\thefigure}{\arabic{section}.\arabic{figure}}
%\renewcommand{\thetable}{\arabic{section}.\arabic{table}}
\makeatletter
\@addtoreset{equation}{section}
\@addtoreset{figure}{section}
\@addtoreset{table}{section}
\makeatother

\renewcommand{\thesection}{\Roman{section}}
\renewcommand{\thesubsection}{\thesection-\Alph{subsection}}

% http://latexcolor.com/
\usepackage{color}
\definecolor{bleudefrance}{rgb}{0.19, 0.55, 0.91}
\definecolor{royalblue}{rgb}{0.25, 0.41, 0.88}

\usepackage{feynmp-auto}%feynman diagram

\usepackage{siunitx}
\sisetup{
  separate-uncertainty = true,
  table-number-alignment = center,
  table-align-text-post = false,
  retain-zero-uncertainty = true,
}

\renewcommand{\topfraction}{0.9}      % Allow 90% of the first page to be floats
\renewcommand{\textfraction}{0.1}     % Allow only 10% text on a page with floats
\renewcommand{\floatpagefraction}{0.5}% Don't require floats to fill the whole page to 
